# Supplementary material for: Moir\'e-driven multiferroic order in twisted CrCl$_3$, CrBr$_3$ and CrI$_3$ bilayers
Source: arXiv:2207.01416 source file (2023-04-16)
Supplement: Supplementary file 1 [file Supplemental_Material.pdf]

# Supplemental Material: Moiré-driven multiferroic order in twisted $CrCl_3$, $CrBr_3$ and $CrI_3$ bilayers

Adolfo O. Fumega[1] and Jose L. Lado[1]

[1] *Department of Applied Physics, Aalto University, 02150 Espoo, Finland*

## COMPUTATIONAL METHODS

### Non-collinear Density Functional Theory calculations

*Ab initio* density functional theory calculations were carried out with the all-electron full-potential linearized augmented-plane-wave method, using a fully non-collinear formalism with spin-orbit coupling (SOC) as implemented in Elk[1] that allows us to treat spin textures. This kind of non-collinear calculations make use of fictitious external magnetic fields applied throughout the muffin-tin spheres. The fields are only used to break the spin symmetry in the first iteration, and switched off afterwards. Therefore, these fictitious fields to not change the results of the calculations. This is known as the Kubler's trick [2]. We have used the local density approximation (LDA) for the exchange correlation functional [3]. In this non-collinear formalism, LDA is the most common exchange correlation functional due to its simple implementation of the non-collinear formalism compared to other exchange correlation functionals [1, 4, 5]. Moreover, our DFT calculations are performed to quantify the effect of the inverse Dzyaloshinskii-Moriya interaction for a given spin texture in the family of chromium trihalides. This interaction depends on both the spin texture and the strength of the spin orbit coupling present in the system. Therefore, a substantial change in the results is not expected from the exchange correlation functional.

The results presented in the manuscript are converged concerning all the parameters. Calculations of the different magnetic configurations require careful convergence of the total electron density: with a $480 \times 60$ real space mesh for the electronic density and a convergence of the Kohn-Sham potential of $10^{-7}$ a.u. for the ferrooelectric forces.

### Ground state of the spin Hamiltonian

The ground state spin configuration was obtained by minimizing the total energy using the Broyden–Fletcher–Goldfarb–Shanno algorithm minimization with the Scipy Python library[6]. This is a gradient descendant algorithm that allows to find the energy minimum by determining the descent direction with a by preconditioning of the gradient with the curvature of the energy functional. The Hessian matrix of the energy functional is obtained from gradient evaluations via a generalized secant method. The gradient is explicitly evaluated via differential programming with JAX[7]. A random initialization of the parameters was considered to find the ground state configuration, and we verified that different random initializations lead to equivalent ground state configurations.

### Interlayer magnetic exchange parametrization

The site dependency of the interlayer exchange $J(\mathbf{r}_i, \mathbf{r}_j)$ was modeled by doing an interpolation with harmonic functions between the antiferromagnetic monoclinic and ferromagnetic rhombohedral regions in an analogous way to the one presented in Refs. [8–10]. We note that our functional form for the interlayer exchange automatically accounts for the spatial dependence created by the moiré. Therefore, the site dependence parametrization of $J_M(\mathbf{r})$ is analytically built as an expansion with harmonic function that preserves the $C_3$ symmetry of the moiré lattice

$$J_M(\mathbf{r}) = \sum_\alpha B_\alpha \cos\left(\mathbf{k}_\alpha \cdot \mathbf{r} + \varphi_\alpha\right) \quad (1)$$

where $B_\alpha$ are the coefficients of the expansion, $\mathbf{k}_\alpha$ are the wave vectors of the expansion with wave length shorter than the moiré length, $\varphi_\alpha$ is a phase and $\mathbf{r}$ correspond to the real space vector describing the coordinates in the moiré unit cell. To get the neighboring interlayer exchange $J(\mathbf{r}_i, \mathbf{r}_j)$ between different moiré sites $\mathbf{r}_j$ and $\mathbf{r}_i$, an average between the $J_M(\mathbf{r})$ of each site is taken and weighted by and exponential factor that controls the length range between neighbors through a $\beta$ parameter as:

$$J_M(\mathbf{r}_i, \mathbf{r}_j) = \frac{J_M(\mathbf{r}_j) + J_M(\mathbf{r}_i)}{2} e^{-\beta(\mathbf{r}_j - \mathbf{r}_i)^2} \quad (2)$$

We can modify the weights in this expansion to demonstrate the robustness of our results against perturbations of the interlayer exchange.

Figure S1a shows the profiles for three different parametrizations in which the weights in the harmonic expansion have been modified. This was performed in such a way that the ratio between antiferromagnetic (monoclinic M) and the two ferromagnetic exchanges in

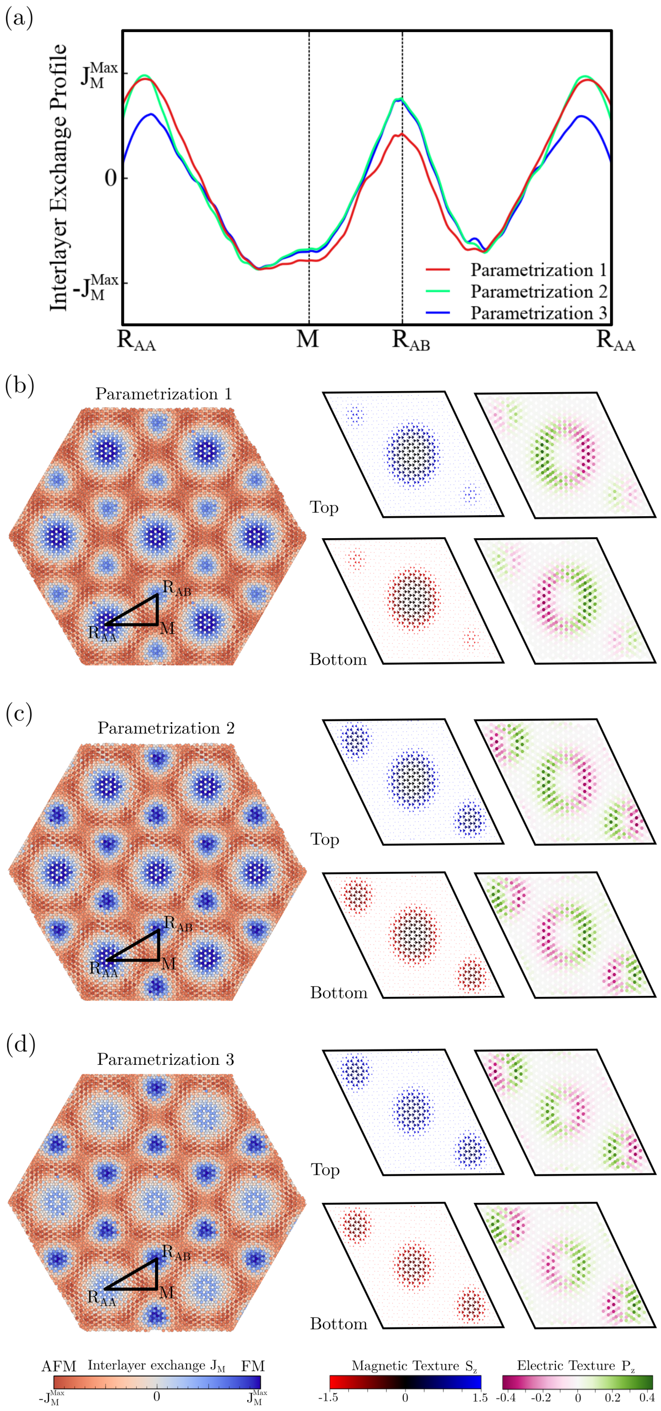


FIG. S1. (a) Interlayer exchange profiles for three different parametrizations of $J_M(\mathbf{r}_i, \mathbf{r}_j)$ following the triangular path shown in the moiré patterns of panels (b,c,d). The ration between antiferromagnetic (monoclinic M) and the two ferromagnetic exchanges in these (rhombohedral $R_{AA}$ and $R_{AB}$) regions changes. Panels (b,c,d) correspond to the site-dependent moiré interlayer exchanges $J_M(\mathbf{r}_i, \mathbf{r}_j)$ and their corresponding ground spin texture and associated electric polarization for parametrizations 1, 2 and 3 respectively.

these (rhombohedral $R_{AA}$ and $R_{AB}$) regions changes.

Figs. S1b, S1c and S1d show the moiré dependence of the interlayer exchanges $J_M(\mathbf{r}_i, \mathbf{r}_j)$ for each parametrization and their corresponding ground state spin textures and associated electric dipoles. We can observe that as long as the antiferromagnetic and ferromagnetic regions are preserved in the twisted system, the non-topological ground state spin texture analyzed in this study emerges. Therefore, this demonstrates a robust behavior against changes in the interlayer exchange parametrization and to small physical perturbations that could arise due to atomic relaxations occurring in the moiré system. Finally, in our calculations, we have fixed the twist angle to 2.64°, which corresponds to an 11×11 commensurate supercell. In previous experiments and theoretical works, it is found that antiferromagnetic and ferromagnetic regions coexist and form non-collinear textures for twisting angles lower than 3°. Here, we have corroborated that the formation of non-collinear magnetic textures is robust against perturbations to the interlayer moiré magnetic exchange. This is effectively equivalent to introduce perturbations on the twisting angle. No qualitative change is observed in the results of our analyses for small variations of the twist angle. Therefore, these results together demonstrate that the physical phenomenology studied in this work would be obtained for twisting angles lower than 3°.

## DISCUSSION ABOUT THE PARAMETERS ENTERING THE SPIN HAMILTONIAN

The conclusions about the multiferroic order strength are made considering values of $J_M^{max}/J = 0.1$, which is typical order of magnitude for the family of $CrX_3$ found in experiments[11, 12]. Higher values such as those obtained by applying uniaxial pressure[13–16] would produce a stronger multiferroic order. Note also that DFT calculations tend to overestimate interlayer exchange, providing values one or two orders of magnitude higher than the ones found experimentally [8, 9]. For the anisotropic magnetic exchange $A_v$, we have considered previous DFT calculations and experiments that have independently predicted values on the order of $A_v \approx 0.1$ meV for $CrI_3$, $A_v \approx 0.01$ meV for $CrBr_3$ and $A_v \approx 0.001$ meV for $CrCl_3$ and for the first neighbor Heisenberg exchange $J$ on the order 2-3 meV [8, 9, 17–20]

## OTHER SOURCES OF MULTIFERROICITY AND MAGNETOELECTRIC COUPLING

### The ferroelectric sliding effect

The sliding ferroelectricity that might occur in twisting bilayers has not been considered as a source for ferroelectricity in our analyses in the main manuscript. This slid-

ing ferroelectric effect is purely structural, meaning that it does not stem from an underlying magnetic order. This has two major consequences. First, the ferroelectricity presented in the main manuscript as a consequence of the inverse DM would vanish above the magnetic transition temperature, in contrast with the sliding ferroelectric effect. Furthermore, changes in the magnetic arrangement in the twisted bilayer will switch the sign of the ferroelectric order. This implies that the ferroelectric order presented in the main text can be controlled with an external magnetic field due to the strong magnetoelectric coupling, in contrast with the ferroelectric sliding effect.

### Discussion about topological magnetoelectric couplings

Note that the skyrmionic phases presented in the main manuscript are electrically achieved through the magnetoelectric coupling produced by the inverse DM interaction in the topologically-trivial ground state spin texture displayed by the twisted magnets. The emergence of magnetic skyrmions will introduce intrinsic topological magnetoelectric couplings [21, 22] that will add on top of this conventional one, and they have not been considered here.


[1] "Elk code," http://elk.sourceforge.net/.
[2] J Kubler, K-H Hock, J Sticht, and A R Williams, "Density functional theory of non-collinear magnetism," Journal of Physics F: Metal Physics **18**, 469 (1988).
[3] J. P. Perdew and Alex Zunger, "Self-interaction correction to density-functional approximations for many-electron systems," Phys. Rev. B **23**, 5048–5079 (1981).
[4] Stanislav Komorovsky, Peter J. Cherry, and Michal Repisky, "Four-component relativistic time-dependent density-functional theory using a stable noncollinear dft ansatz applicable to both closed- and open-shell systems," The Journal of Chemical Physics **151**, 184111 (2019), https://doi.org/10.1063/1.5121713.
[5] Zhichen Pu, Ning Zhang, Hong Jiang, and Yunlong Xiao, "Approach for noncollinear gga kernels in closed-shell systems," Phys. Rev. B **105**, 035114 (2022).
[6] "Scipy python library," https://scipy.org/.
[7] "Jax," https://github.com/google/jax.
[8] Feiping Xiao, Keqiu Chen, and Qingjun Tong, "Magnetization textures in twisted bilayer $crx_3$ (x=br, i)," Phys. Rev. Research **3**, 013027 (2021).
[9] Muhammad Akram, Harrison LaBollita, Dibyendu Dey, Jesse Kapeghian, Onur Erten, and Antia S. Botana, "Moiré skyrmions and chiral magnetic phases in twisted $CrX_3$ (x = i, br, and cl) bilayers," Nano Letters **21**, 6633–6639 (2021).
[10] Nikhil Sivadas, Satoshi Okamoto, Xiaodong Xu, Craig. J. Fennie, and Di Xiao, "Stacking-dependent magnetism in bilayer $CrI_3$," Nano Letters **18**, 7658–7664 (2018).
[11] D. R. Klein, D. MacNeill, J. L. Lado, D. Soriano, E. Navarro-Moratalla, K. Watanabe, T. Taniguchi, S. Manni, P. Canfield, J. Fernández-Rossier, and P. Jarillo-Herrero, "Probing magnetism in 2d van der waals crystalline insulators via electron tunneling," Science **360**, 1218–1222 (2018).
[12] Tiancheng Song, Qi-Chao Sun, Eric Anderson, Chong Wang, Jimin Qian, Takashi Taniguchi, Kenji Watanabe, Michael A. McGuire, Rainer Stöhr, Di Xiao, Ting Cao, Jörg Wrachtrup, and Xiaodong Xu, "Direct visualization of magnetic domains and moiré magnetism in twisted 2d magnets," Science **374**, 1140–1144 (2021).
[13] Tiancheng Song, Zaiyao Fei, Matthew Yankowitz, Zhong Lin, Qianni Jiang, Kyle Hwangbo, Qi Zhang, Bosong Sun, Takashi Taniguchi, Kenji Watanabe, Michael A. McGuire, David Graf, Ting Cao, Jiun-Haw Chu, David H. Cobden, Cory R. Dean, Di Xiao, and Xiaodong Xu, "Switching 2d magnetic states via pressure tuning of layer stacking," Nature Materials **18**, 1298–1302 (2019).
[14] Tingxin Li, Shengwei Jiang, Nikhil Sivadas, Zefang Wang, Yang Xu, Daniel Weber, Joshua E. Goldberger, Kenji Watanabe, Takashi Taniguchi, Craig J. Fennie, Kin Fai Mak, and Jie Shan, "Pressure-controlled interlayer magnetism in atomically thin CrI3," Nature Materials **18**, 1303–1308 (2019).
[15] Matthew Yankowitz, Shaowen Chen, Hryhoriy Polshyn, Yuxuan Zhang, K. Watanabe, T. Taniguchi, David Graf, Andrea F. Young, and Cory R. Dean, "Tuning superconductivity in twisted bilayer graphene," Science **363**, 1059–1064 (2019).
[16] Adolfo O. Fumega, S. Blanco-Canosa, H. Babu-Vasili, P. Gargiani, Hongze Li, Jian-Shi Zhou, F. Rivadulla, and Victor Pardo, "Electronic structure and magnetic exchange interactions of cr-based van der waals ferromagnets. a comparative study between crbr3 and cr2ge2te6," J. Mater. Chem. C **8**, 13582–13589 (2020).
[17] J L Lado and J Fernández-Rossier, "On the origin of magnetic anisotropy in two dimensional $CrI_3$," 2D Materials **4**, 035002 (2017).
[18] Wei-Bing Zhang, Qian Qu, Peng Zhu, and Chi-Hang Lam, "Robust intrinsic ferromagnetism and half semiconductivity in stable two-dimensional single-layer chromium trihalides," Journal of Materials Chemistry C **3**, 12457–12468 (2015).
[19] Kok Wee Song and Vladimir I Fal'ko, "Superexchange and Spin-Orbit Coupling in Mono and Bilayer Chromium Trihalides," arXiv e-prints , arXiv:2207.00365 (2022), arXiv:2207.00365 [cond-mat.str-el].
[20] Thomas A. Tartaglia, Joseph N. Tang, Jose L. Lado, Faranak Bahrami, Mykola Abramchuk, Gregory T. McCandless, Meaghan C. Doyle, Kenneth S. Burch, Ying Ran, Julia Y. Chan, and Fazel Tafti, "Accessing new magnetic regimes by tuning the ligand spin-orbit coupling in van der waals magnets," Science Advances **6** (2020), 10.1126/sciadv.abb9379.
[21] Börge Göbel, Alexander Mook, Jürgen Henk, and Ingrid Mertig, "Magnetoelectric effect and orbital magnetization in skyrmion crystals: Detection and characterization of skyrmions," Phys. Rev. B **99**, 060406 (2019).
[22] Sayantika Bhowal and Nicola A. Spaldin, "Magnetoelectric classification of skyrmions," Phys. Rev. Lett. **128**, 227204 (2022).
